# Supplementary material for: Controlling the position of traveling waves in reaction-diffusion systems
Source: arXiv:1304.2327 ancillary file (2014-01-17)
Supplement: Supplementary file 1 [file Supplement.pdf]

# Controlling the position of traveling waves in reaction-diffusion systems - Supplemental material

Jakob Löber* and Harald Engel

*Institut für Theoretische Physik, EW 7-1, Technische Universität Berlin, Hardenbergstraße 36, 10623 Berlin, Germany*

In this supplement, we present additional figures and information on the chosen parameter values for numerical simulations as well as details of derivations. Each figure is associated with a movie which can be found in the supplementary material.

In section I we show that a control of traveling waves (TW) acting via the translational mode related to the spatial invariance of the uncontrolled reaction-diffusion system (RDS) shifts the wave as a whole while it preserves its profile. Section II and III present additional numerical details for position control of a Schlögl front solution via a multiplicatively coupled control function and for an additive position control of a solitary FitzHugh-Nagumo pulse, respectively. In the next section IV we consider the traveling front solution to the Fisher equation as a representative example for a traveling wave solution which does not exhibit a spectral gap. We find that under an additive position control deviations from the uncontrolled wave profile grow unboundedly, while the control is successful if it couples multiplicatively with the RDS. A generalization of our method for non-invertible coupling matrices to RDS of Hodgkin-Huxley type is given in section V. Two cases are elaborated that might be of interest for possible applications. Either only the transmembrane potential or only one of the gating variables are accessible to the control. In two separate sections VI and VII, we study the application of position control to the photosensitive Belousov-Zhabotinsky (BZ) reaction. Based on the modified Oregonator model we derive explicit analytical expressions for the spatio-temporal variation of the applied light intensity to realize position control of chemical waves in the BZ reaction, which one can check experimentally. We also show an example for which position control fails. In section VIII we conclude with additional details on the derivations and numerical simulations of stationary control.

## I. CONTROLS REALIZING A GENERAL PROTOCOL OF MOVEMENT

In this section we show that a perturbation proportional to the Goldstone mode shifts a TW solution and simultaneously preserves the unperturbed wave profile. We consider a perturbed RDS with $n$ components

$$\mathbf{u} = \mathbf{u}(x,t) = (u_1(x,t), \ldots, u_n(x,t))^T \quad \text{(S1)}$$

(superscripted $T$ denotes transpose) of the form

$$\partial_t \mathbf{u} = D\partial_x^2 \mathbf{u} + \mathbf{R}(\mathbf{u}) + \epsilon \mathbf{f}(x,t). \quad \text{(S2)}$$

We assume that the TW $\mathbf{U}_c(x-ct)$ is a solution of the unperturbed ($\epsilon = 0$) case. With the ansatz

$$\mathbf{u}(x,t) = \mathbf{U}_c(x-ct) + \epsilon \mathbf{v}(x,t) \quad \text{(S3)}$$

we find in order $\mathcal{O}(\epsilon)$ in the comoving frame $\xi = x - ct$ a linear partial differential equation (PDE) for $\hat{\mathbf{v}}(\xi,t) = \hat{\mathbf{v}}(x-ct,t) = \mathbf{v}(x,t)$ with inhomogeneity $\hat{\mathbf{f}}(\xi,t) = \mathbf{f}(\xi+ct,t) = \mathbf{f}(x,t)$,

$$\partial_t \hat{\mathbf{v}}(\xi,t) = \mathcal{L}\hat{\mathbf{v}}(\xi,t) + \hat{\mathbf{f}}(\xi,t), \quad \text{(S4)}$$

$$\mathcal{L} = D\partial_\xi^2 + c\partial_\xi + \mathcal{D}\mathbf{R}(\mathbf{U}_c(\xi)). \quad \text{(S5)}$$

The matrix $\mathcal{D}\mathbf{R}(\mathbf{U}_c(\xi))$ denotes the Jacobi matrix of the nonlinear reaction function $\mathbf{R}$ evaluated at the TW solution $\mathbf{U}_c(\xi)$. The initial and boundary conditions, respectively, for $\hat{\mathbf{v}}$ are

$$\hat{\mathbf{v}}(\xi,0) = 0, \quad \text{(S6)}$$

$$\lim_{\xi\to\pm\infty} \hat{\mathbf{v}}(\xi,t) = 0. \quad \text{(S7)}$$

We denote the eigenvalues of $\mathcal{L}$ as $\lambda_i$ and the corresponding eigenfunctions as $\mathbf{w}_i(\xi)$,

$$\mathcal{L}\mathbf{w}_i(\xi) = \lambda_i \mathbf{w}_i(\xi). \quad \text{(S8)}$$

The TW $\mathbf{U}_c(\xi)$ is assumed to be stable such that all eigenvalues $\lambda_i$ have real part smaller than or equal to zero. The Goldstone mode is the eigenfunction $\mathbf{w}_0(\xi) = \mathbf{U}_c'(\xi)$ to the eigenvalue with largest real part $\lambda_0 = 0$. We assume that $\lambda_0$ is nondegenerate and that it is the unique eigenvalue with zero real part. Laplace transforming Eq. (S4) with respect to time $t$ and applying the initial condition Eq. (S6) for $\hat{\mathbf{v}}$ yields

$$s\tilde{\mathbf{v}}(\xi,s) = \mathcal{L}\tilde{\mathbf{v}}(\xi,s) + \tilde{\mathbf{f}}(\xi,s), \quad \text{(S9)}$$

xwhere $\tilde{\mathbf{v}}$ and $\tilde{\mathbf{f}}$ are the Laplace transforms of $\hat{\mathbf{v}}$ and $\hat{\mathbf{f}}$, respectively. We assume that a complete orthogonal set of eigenfunctions $\mathbf{w}_i(\xi)$ of the operator $\mathcal{L}$ exists and expand both $\tilde{\mathbf{v}}$ and $\tilde{\mathbf{f}}$ in terms of $\mathbf{w}_i(\xi)$,

$$\tilde{\mathbf{v}}(\xi,s) = \sum_i \tilde{a}_i(s)\mathbf{w}_i(\xi), \quad \text{(S10)}$$

$$\tilde{\mathbf{f}}(\xi,s) = \sum_i \tilde{b}_i(s)\mathbf{w}_i(\xi). \quad \text{(S11)}$$

*jakob@physik.tu-berlin.de

The expansion coefficients $\tilde{a}_i$ and $\tilde{b}_i$ are given in terms of the eigenfunctions $\mathbf{w}_i^\dagger(\xi)$ of the adjoint operator $\mathcal{L}^\dagger$ of $\mathcal{L}$,

$$\mathcal{L}^\dagger = D\partial_\xi^2 - c\partial_\xi + \mathcal{D}\mathbf{R}\left(\mathbf{U}_c(\xi)\right)^T. \tag{S12}$$

The form of $\mathcal{L}^\dagger$ can be found by partial integral with respect to the standard inner product in function space ($\bar{z}$ denotes complex conjugate),

$$\left\langle \mathbf{f}(\xi), \mathbf{g}(\xi)\right\rangle = \int_{-\infty}^{\infty} d\xi \bar{\mathbf{f}}^T(\xi)\,\mathbf{g}(\xi), \tag{S13}$$

such that

$$\left\langle \mathbf{f}(\xi), \mathcal{L}\mathbf{g}(\xi)\right\rangle = \left\langle \mathcal{L}^\dagger\mathbf{f}(\xi), \mathbf{g}(\xi)\right\rangle \tag{S14}$$

for arbitrary functions $\mathbf{f}$ and $\mathbf{g}$. The expression $\mathbf{f}^T(\xi)\,\mathbf{g}(\xi)$ denotes the inner product in the vector space of $n$-dimensional component vectors,

$$\bar{\mathbf{f}}^T(\xi)\,\mathbf{g}(\xi) = \sum_{i=1}^{n} \bar{f}_i(\xi)\, g_i(\xi). \tag{S15}$$

The expansion coefficients $\tilde{a}_i$, $\tilde{b}_i$ are given by

$$\tilde{a}_i(s) = \frac{1}{K_i}\left\langle \mathbf{w}_i^\dagger(\xi), \tilde{\mathbf{v}}(\xi,s)\right\rangle, \tag{S16}$$

$$\tilde{b}_i(s) = \frac{1}{K_i}\left\langle \mathbf{w}_i^\dagger(\xi), \tilde{\mathbf{f}}(\xi,s)\right\rangle. \tag{S17}$$

We assumed that the eigenfunctions $\mathbf{w}_i^\dagger(\xi)$ and $\mathbf{w}_i(\xi)$ constitute an orthogonal set but are not necessarily normalized. The normalization constants are given by

$$\left\langle \mathbf{w}_i^\dagger(\xi), \mathbf{w}_j(\xi)\right\rangle = K_i\delta_{ij}. \tag{S18}$$

Using the expansion Eqs. (S10), (S11) in Eq. (S9), we find

$$\sum_i s\tilde{a}_i(s) = \sum_i \left(\lambda_i\tilde{a}_i(s) + \tilde{b}_i(s)\right) \tag{S19}$$

or

$$\tilde{a}_i(s) = \frac{\tilde{b}_i(s)}{s-\lambda_i}. \tag{S20}$$

The solution $\tilde{\mathbf{v}}$ can be expressed as

$$\begin{aligned}\tilde{\mathbf{v}}(\xi,s) &= \sum_i \tilde{a}_i(s)\,\mathbf{w}_i(\xi)\\ &= \sum_i \frac{\tilde{b}_i(s)}{s-\lambda_i}\mathbf{w}_i(\xi).\end{aligned} \tag{S21}$$

Applying the inverse Laplace transform to $\tilde{\mathbf{v}}(\xi,s)$, we find the solution $\hat{\mathbf{v}}(\xi,t)$ in the time domain

$$\hat{\mathbf{v}}(\xi,t) = \sum_i a_i(t)\,\mathbf{w}_i(\xi), \tag{S22}$$

as a superposition of eigenfunctions $\mathbf{w}_i(\xi)$. The expansion coefficients $a_i(t)$ are determined as

$$a_i(t) = \int_0^t d\tilde{t}e^{\lambda_i(t-\tilde{t})}b_i(\tilde{t}), \tag{S23}$$

and the expansion coefficient $b_i(t)$ is a functional involving the eigenfunction $\mathbf{w}_i^\dagger(\xi)$ of the adjoint operator $\mathcal{L}^\dagger$,

$$\begin{aligned}b_i(t) &= \frac{1}{K_i}\left\langle \mathbf{w}_i^\dagger(\xi), \hat{\mathbf{f}}(\xi,t)\right\rangle\\ &= \frac{1}{K_i}\int_{-\infty}^{\infty} d\xi\bar{\mathbf{w}}_i^{\dagger T}(\xi)\,\hat{\mathbf{f}}(\xi,t)\\ &= \frac{1}{K_i}\int_{-\infty}^{\infty} d\xi\bar{\mathbf{w}}_i^{\dagger T}(\xi)\,\mathbf{f}(x+ct,t).\end{aligned} \tag{S24}$$

Now we can determine the effect of a perturbation $\mathbf{f}$ proportional to the Goldstone mode $\mathbf{U}_c'$,

$$\mathbf{f}(x,t) \sim \mathbf{U}_c'(x-ct), \tag{S25}$$

onto the TW solution $\mathbf{U}_c(\xi)$. Because of the assumed orthogonality of eigenfunctions, it follows immediately for the expansion coefficients

$$b_i(t) = \frac{1}{K_i}\left\langle \mathbf{w}_i^\dagger(\xi), \hat{\mathbf{f}}(\xi,t)\right\rangle = 0,\ i>0 \tag{S26}$$

The only nonzero expansion coefficient is $b_0(t)$. It follows that the solution for $\hat{\mathbf{v}}(\xi,t)$ is proportional to the Goldstone mode,

$$\hat{\mathbf{v}}(\xi,t) = p\mathbf{U}_c'(\xi), \tag{S27}$$

where we denoted the proportionality coefficient by $p$. The full solution for $\mathbf{u}(x,t)$ under the assumed small perturbation proportional to the Goldstone mode is

$$\begin{aligned}\mathbf{u}(x,t) &= \mathbf{U}_c(x-ct) + \epsilon\mathbf{v}(x,t)\\ &= \mathbf{U}_c(x-ct) + \epsilon p\mathbf{U}_c'(x-ct)\\ &\approx \mathbf{U}_c(x-ct+\epsilon p).\end{aligned} \tag{S28}$$

Thus we showed that a perturbation proportional to the Goldstone mode $\mathbf{U}_c'(x-ct)$ leads to a slightly shifted TW while it prevents deformations of the unperturbed wave profile $\mathbf{U}_c(x-ct)$. See Ref. [1] for the derivation of the equation of motion, Eq. (4) of the main text.

## II. MULTIPLICATIVE POSITION CONTROL OF A SCHLÖGL FRONT

The reaction function $R(u)$ of the Schlögl model is a cubic polynomial which can be written in terms of the three ordered roots $u_1$, $u_2$, $u_3$ of $R(u)$

$$R(u) = -(u-u_1)(u-u_2)(u-u_3),\ u_1<u_2<u_3. \tag{S29}$$

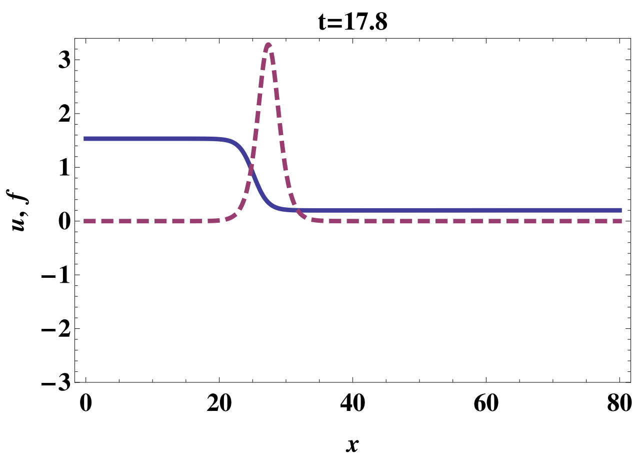


Figure S1. **S1.avi:** Multiplicative position control of the Schlögl front solution (blue solid line). The spatio-temporal control $f(x,t)$ (purple dashed line) couples to the quadratic term $u^2$ in the Schlögl model. The front is moved back and forth with a maximum enforced velocity approximately 10 times larger than the velocity $c$ of the uncontrolled front.

From the chemical reaction mechanism [2], we obtain the the following form of the reaction function

$$R(u) = C_1 u^2 - u^3 - u + C_2. \tag{S30}$$

The parameter values chosen for numerical simulations are

$$C_1 = 2.133, \qquad C_2 = 0.123, \tag{S31}$$
$$D = 1.0. \tag{S32}$$

The velocity $c$ of the unperturbed TW is

$$c = \sqrt{\frac{D}{2}}\left(u_1 + u_3 - 2u_2\right) = 0.662. \tag{S33}$$

The protocol for a sinusoidal movement with period $T$ and amplitude $A$ reads

$$\phi(t) = A_0 + A \sin\left(\frac{2\pi t}{T} + A_1\right). \tag{S34}$$

The protocol parameters $A_0$ and $A_1$ are determined from the condition that the protocol is smooth at the initial time $t = t_0$,

$$\phi(t_0) = \phi_0, \qquad \dot{\phi}(t_0) = c, \tag{S35}$$

leading to the result

$$A_0 = A\sqrt{1 - \frac{c^2T^2}{4A^2\pi^2}} + \phi_0, \tag{S36}$$
$$A_1 = -\frac{2\pi t_0}{T} - \operatorname{arcsec}\left(\frac{2\pi A}{cT}\right). \tag{S37}$$

Results obtained for the parameters and initial conditions

$$A = 15, \qquad T = 12, \tag{S38}$$
$$t_0 = 5, \qquad \phi_0 = c t_0 = 3.3. \tag{S39}$$

are shown in the snapshot at time $t = 17.8$, Fig. S1, and the corresponding movie.

## III. CONTROLLING THE POSITION OF A FITZHUGH-NAGUMO PULSE

The FitzHugh-Nagumo (FHN) model equations [3] are

$$\partial_t u = D_u \partial_x^2 u + 3u - u^3 - v + \epsilon\left(\mathcal{G}_{11} f_u + \mathcal{G}_{12} f_v\right), \tag{S40}$$
$$\partial_t v = D_v \partial_x^2 v + \tilde{\epsilon}\left(u - \delta\right) - \gamma v + \epsilon\left(\mathcal{G}_{21} f_u + \mathcal{G}_{22} f_v\right). \tag{S41}$$

We choose for the parameter values

$$\delta = -1.3, \qquad \tilde{\epsilon} = 0.33, \tag{S42}$$
$$D_u = 1.0, \qquad D_v = 0.3, \tag{S43}$$
$$\gamma = 0, \qquad \epsilon = 1, \tag{S44}$$

and for the coupling matrix

$$\mathcal{G} = \begin{pmatrix} \mathcal{G}_{11} & \mathcal{G}_{12} \\ \mathcal{G}_{21} & \mathcal{G}_{22} \end{pmatrix} = \begin{pmatrix} 1 & 0 \\ 1/2 & 1 \end{pmatrix}. \tag{S45}$$

No exact analytical solution for the pulse profile $\mathbf{U}_c$ and the velocity $c$ of the FHN model is known. Therefore, we obtain the pulse profile and the velocity from numerical simulations of the uncontrolled FHN model. An interpolated version of the pulse profile is then used to compute the derivative $\mathbf{U}_c'(x)$ necessary for the control function. The velocity $c$ of the uncontrolled TW determined from numerical simulations is

$$c = 1.165. \tag{S46}$$

A protocol accelerating the pulse is

$$\phi(t) = ct\left(1 + \alpha t/T\right). \tag{S47}$$

During the time interval $T$, the wave is accelerated to a velocity $1 + 2\alpha$ times larger than the velocity $c$ of the unperturbed wave. We set

$$T = 30, \qquad \alpha = 7.5. \tag{S48}$$

See the snapshot Fig. S2 and corresponding movie for the results of numerical simulations and a comparison with optimal control.
For the case that the control acts solely on the activator equation,

$$\partial_t u = D_u \partial_x^2 u + 3u - u^3 - v + \epsilon \tilde{f}_u, \tag{S49}$$
$$\partial_t v = D_v \partial_x^2 v + \tilde{\epsilon}\left(u - \delta\right) - \gamma v, \tag{S50}$$

we choose a protocol

$$\phi(t) = ct + A\left(\cos\left(\frac{2\pi t}{T}\right) - 1\right) \tag{S51}$$

with

$$A = 60, \qquad T = 20. \tag{S52}$$

All other parameter values are the same as stated above. The control function $\tilde{f}_u$ is given as

$$\tilde{f}_u(x,t) = -\mathcal{K} f_v + f_u, \tag{S53}$$

while $f_u$ and $f_v$ are

$$f_u(x,t) = \left(c - \dot{\phi}(t)\right) U_c'(x - \phi(t)), \tag{S54}$$

$$f_v(x,t) = \left(c - \dot{\phi}(t)\right) V_c'(x - \phi(t)), \tag{S55}$$

with $U_c(x)$ and $V_c(x)$ the TW profiles of the uncontrolled FHN model. The term $a(x,t) = \mathcal{K} f_v(x,t)$ involving the operator $\mathcal{K}$ can be obtained as the solution to the PDE

$$\partial_t a(x,t) - D_v \partial_x^2 a(x,t) + \tilde{\epsilon}\gamma a(x,t) = f_v(x,t), \tag{S56}$$

$$a(x,t_0) = 0. \tag{S57}$$

See the snapshot Fig. S3 and corresponding movie.

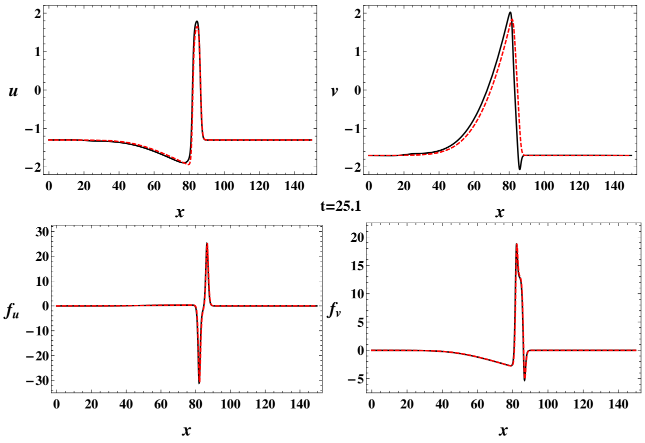


Figure S2. **S2.avi:** Comparison of optimal (red dashed) and analytical control (black solid) of a stable FitzHugh-Nagumo pulse. Top: The activator $u$ (left) and inhibitor $v$ (right) of the controlled pulse solution. Bottom: Control functions $f_u$ (left) and $f_v$ (right) acting on activator and inhibitor via the coupling matrix $\mathcal{G}$. The propagation velocity of the pulse is increased up to 16 times the velocity $c$ of the uncontrolled pulse while the pulse profile is only slightly deformed.

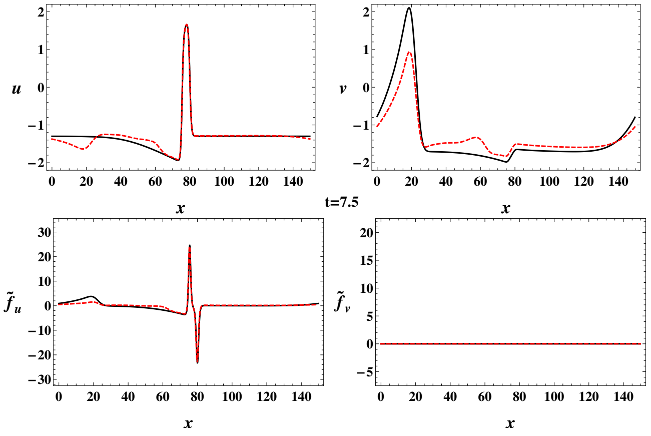


Figure S3. **S3.avi:** Top: The activator $u$ (left) and inhibitor $v$ (right) of the controlled FitzHugh-Nagumo equations. Bottom: The control functions $\tilde{f}_u$ (left) acts on the activator while the control function $\tilde{f}_v$ (right) acting on the inhibitor is zero.

## IV. POSITION CONTROL OF THE FRONT SOLUTION TO THE FISHER EQUATION

The logistic growth model for a number $N$ of individuals of a population is

$$\dot{N}(t) = rN(t)\left(1 - \frac{N(t)}{K}\right), \tag{S58}$$

where $K$ is the carrying capacity, i.e. the number of individuals an environment can sustain, and $r$ the growth rate of the population [4]. Rescaling Eq. (S58) and including diffusion leads to the Fisher or Kolmogorov-Petrovsky-Piskunov (KPP) equation [5, 6]

$$\partial_t u = \partial_x^2 u + u(1-u) + \epsilon f(x,t). \tag{S59}$$

We added a source term $f$ which we assume can be controlled in a spatio-temporal way. The unperturbed ($\epsilon = 0$) Eq. (S59) has a one parameter family of monotonously decreasing unstable front solutions $U_c$ with velocity $c > 2$. The front solution with velocity $c = 2$ is marginally stable, meaning that the continuous spectrum of $\mathcal{L}$ reaches up to the origin of the complex plane and there is no spectral gap [7, 8].
We choose a protocol which changes the velocity from the initial value $c$ to the final velocity $c_1$,

$$\dot{\phi}(t) = \frac{(c - c_1)}{2}\left(\cos\left(\pi\frac{t - t_0}{t_1 - t_0}\right) + 1\right) + c_1. \tag{S60}$$

Integration and enforcing the initial condition $\phi(t_0) = \phi_0$ yields

$$\phi(t) = \phi_0 + \frac{1}{2}(c + c_1)(t - t_0) - \frac{1}{2\pi}(c_1 - c_0)(t_1 - t_0)\sin\left(\pi\frac{t - t_0}{t_1 - t_0}\right). \tag{S61}$$

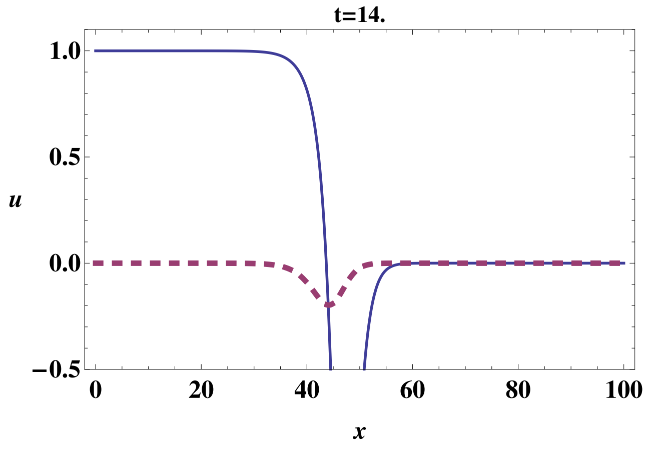


Figure S4. **S4.avi:** Position control of the Fisher front solution (blue solid line) by an additive control (purple dashed line). The control attempts to stop the front but leads to a front profile growing indefinitely to $-\infty$ in the region where the control is large.

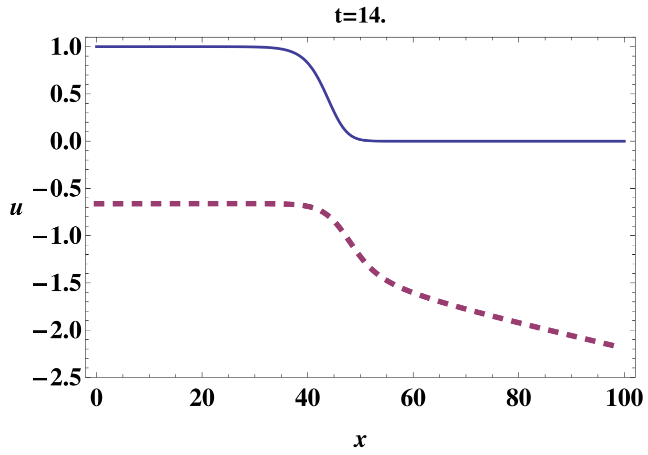


Figure S5. **S5.avi:** Position control of the Fisher front solution (blue solid line) by a control via the growth rate $r$ of the logistic growth model Eq. (S58). The control (purple dashed line) successfully stops the front while it preserves the front profile of the uncontrolled wave.

This protocol ensures that the accelerations at initial time $t_0$ and final time $t_1$ are zero while the velocity is continuously changed from $c$ at the initial time $t = t_0$ to $c_1$ at the final time $t = t_1$,

$$\dot{\phi}(t_0) = c, \qquad \dot{\phi}(t_1) = c_1, \tag{S62}$$

$$\ddot{\phi}(t_0) = 0, \qquad \ddot{\phi}(t_1) = 0. \tag{S63}$$

We choose the protocol parameters such that the front is stopped,

$$c = 2, \qquad t_0 = 0 \tag{S64}$$

$$c_1 = 0, \qquad t_1 = 20. \tag{S65}$$

Applying the additive control

$$f(x,t) = \left(c - \dot{\phi}(t)\right) U_c'(x - \phi(t)) \tag{S66}$$

to the Fisher equation (S59) with the marginally stable Fisher front solution as the initial condition leads to a front profile not traveling any further to the right, but growing instead indefinitely to $-\infty$ in the region where the control is large, see the snapshot Fig. S4 and corresponding movie.
As a second example we consider control by the growth rate $r \to r + \epsilon f(x,t)$ in Eq. (S58). In rescaled form, this leads to a Fisher equation with multiplicative control

$$\partial_t u = \partial_x^2 u + u(1-u) + \epsilon u (1-u) f(x,t). \tag{S67}$$

The solution for the control function is given by

$$f(x,t) = \left(c - \dot{\phi}(t)\right) \frac{U_c'(x-\phi(t))}{U_c(x-\phi(t))(1-U_c(x-\phi(t)))}. \tag{S68}$$

In contrast to the additive control, no instability arises in this case and the control successfully stops the wave front while it preserves the wave profile $U_c$ of the uncontrolled wave, see the snapshot (S5) and corresponding movie. Note that the control is not localized in this case because the denominator behaves as $\lim_{x\to\pm\infty} U_c(x-\phi(t))(1-U_c(x-\phi(t))) = 0$.

## V. DERIVATION OF CONTROL FUNCTIONS FOR HODGKIN-HUXLEY TYPE MODELS

We discuss how control functions can be derived for the class of models given by a RDS with $n+1$ components of the form

$$\partial_t u = D_u \partial_x^2 u + R(u, v_1, \dots, v_n) + \epsilon f_u, \tag{S69}$$

$$\partial_t v_i = D_i \partial_x^2 v_i + g_i(u) + h_i(u) v_i + \epsilon f_i, \; i \in \{1, \dots, n\}. \tag{S70}$$

For the original Hodgkin-Huxley model [9], $u$ denotes the transmembrane potential, i.e. the difference between the interior and exterior cellular electrical potential and $v_1$, $v_2$, $v_3$ are gating variables with zero diffusion coefficients $D_1 = D_2 = D_3 = 0$ which model the dynamics of ion channels. For Eqs. (S69), (S70), the appropriate control functions for position control are given by

$$\begin{pmatrix} f_u \\ f_1 \\ \vdots \\ f_n \end{pmatrix} = \left(c - \dot{\phi}(t)\right) \begin{pmatrix} U_c{}'(x-\phi(t)) \\ V_c^{1\prime}(x-\phi(t)) \\ \vdots \\ V_c^{n\prime}(x-\phi(t)) \end{pmatrix}, \tag{S71}$$

where $U_c(x)$, $V_c^i(x)$ are the TW profiles the uncontrolled RDS, Eqs. (S69), (S70) with $\epsilon = 0$. Equations (S70) for $v_i$ are linear inhomogeneous PDEs

$$\partial_t v_i - D_i \partial_x^2 v_i - h_i(u) v_i = g_i(u) + \epsilon f_i, \tag{S72}$$

with initial conditions

$$v_i(x,t_0) = v_i^0(x). \tag{S73}$$

The solutions $\tilde{v}_i$ to Eq. (S4) are a superposition of the solution to the corresponding inhomogeneous equation with zero initial condition and the solution to the homogeneous equation with initial condition $v_i^0$. In terms of the Green's operators $\mathcal{V}_i^0[u]$ and $\mathcal{V}_i[u]$ the solutions $v_i$ can be written as

$$\tilde{v}_i = \mathcal{V}_i^0[u]\, v_i^0 + \mathcal{V}_i[u]\left(g_i(u) + \epsilon f_i\right). \tag{S74}$$

The operators $\mathcal{V}_i^0[u]$ and $\mathcal{V}_i[u]$ depend on $u$ because in general the functions $h_i$ depend on $u$. The RDS Eqs. (S69),(S70) can be written as a single nonlinear partial Integro-Differential Equation (IDE)

$$\partial_t u = D_u \partial_x^2 u + R(u,\tilde{v}_1,\dots,\tilde{v}_n) + \epsilon f_u, \tag{S75}$$

$$\tilde{v}_i = \underbrace{\mathcal{V}_i^0[u]\, v_i^0 + \mathcal{V}_i[u]\, g_i(u)}_{=\hat{v}_i} + \epsilon \mathcal{V}_i[u]\, f_i. \tag{S76}$$

We defined the $\hat{v}_i$ as that part of solution $\tilde{v}_i$ which does not involve the control term $f_i$. To isolate the control terms, we expand Eq. (S75) for $u$ in $\epsilon$

$$\begin{aligned}\partial_t u = {} & D_u \partial_x^2 u + R(u,\hat{v}_1,\dots,\hat{v}_n) \\ & + \epsilon \sum_{i=1}^n \partial_{\hat{v}_i} R(u,\hat{v}_1,\dots,\hat{v}_n)\, \mathcal{V}_i[u]\, f_i \\ & + \epsilon f_u + \mathcal{O}(\epsilon^2),\end{aligned} \tag{S77}$$

with

$$\partial_{\hat{v}_i} R(u,\hat{v}_1,\dots,\hat{v}_n) = \partial_{v_i} R(u,v_1,\dots,v_n)\Big|_{v_1=\hat{v}_1,\dots,v_n=\hat{v}_n}. \tag{S78}$$

For the case $f_u = \tilde{f}_u$ and $f_i \equiv 0$, $i \in \{1,\dots,n\}$, we have

$$\partial_t u = D_u \partial_x^2 u + R(u,v_1,\dots,v_n) + \epsilon \tilde{f}_u, \tag{S79}$$

$$\partial_t v_i = D_i \partial_x^2 v_i + g_i(u) + h_i(u)\, v_i. \tag{S80}$$

Written as a single IDE, we obtain instead of Eq. (S75)

$$\partial_t u = D_u \partial_x^2 u + R(u,\hat{v}_1,\dots,\hat{v}_n) + \epsilon \tilde{f}_u. \tag{S81}$$

Note that $\tilde{v}_i = \hat{v}_i$ in this case. Comparing the control terms with Eq. (S77), we obtain

$$\tilde{f}_u = f_u + \sum_{i=1}^n \partial_{\hat{v}_i} R(u,\hat{v}_1,\dots,\hat{v}_n)\, \mathcal{V}_i[u]\, f_i, \tag{S82}$$

with $f_i$ from Eq. (S71). Eq. (S82) represents a feedback control because it depends directly and via the $\hat{v}_i$ on the controlled activator variable $u$. If the control is successful, the controlled wave equals approximately the uncontrolled wave profile $\mathbf{U}_c$ shifted according to the protocol and $u = U_c(x-\phi(t)) + \mathcal{O}(\epsilon)$, $v_i = V_c^i(x-\phi(t)) + \mathcal{O}(\epsilon)$ to leading order in $\epsilon$. With $U_c = U_c(x-\phi(t))$, $V_c^i = V_c^i(x-\phi(t))$ we obtain the final result from Eq. (S82)

$$\tilde{f}_u = f_u + \sum_{i=1}^n \partial_{V_c^i} R\left(U_c, V_c^1,\dots,V_c^n\right) \mathcal{V}_i[U_c]\, f_i. \tag{S83}$$

The terms $a_i = \mathcal{V}_i[U_c(x-\phi(t))]\, f_i$ are given as the solutions to the inhomogeneous PDEs (compare Eq. (S70))

$$\partial_t a_i - D_i \partial_x^2 a_i - h_i(U_c(x-\phi(t)))\, a_i = f_i, \tag{S84}$$

$$a_i(x,t_0) = 0. \tag{S85}$$

Next we consider the case that only one of the gating variables $v_i$ can be controlled, say $f_1 = \tilde{f}_1$ is nonzero and all other controls vanish, $f_u \equiv 0$, $f_i \equiv 0$, $i \in \{2,\dots,n\}$. The controlled RDS reads

$$\partial_t u = D_u \partial_x^2 u + R(u,v_1,\dots,v_n), \tag{S86}$$

$$\partial_t v_1 = D_1 \partial_x^2 v_i + g_1(u) + h_1(u)\, v_1 + \epsilon \tilde{f}_1, \tag{S87}$$

$$\partial_t v_i = D_i \partial_x^2 v_i + g_i(u) + h_i(u)\, v_i,\ i \in \{2,\dots,n\}. \tag{S88}$$

Written as a single IDE, we get

$$\begin{aligned}\partial_t u = {} & D_u \partial_x^2 u + R(u,\hat{v}_1,\dots,\hat{v}_n) \\ & + \epsilon \partial_{\hat{v}_1} R(u,\hat{v}_1,\dots,\hat{v}_n)\, \mathcal{V}_1[u]\, \tilde{f}_1.\end{aligned} \tag{S89}$$

Comparing the control terms with Eq. (S77) gives

$$\partial_{\hat{v}_1} R(u,\hat{v}_1,\dots,\hat{v}_n)\, \mathcal{V}_1[u]\, \tilde{f}_1 \tag{S90}$$

$$= \sum_{i=1}^n \partial_{\hat{v}_i} R(u,\hat{v}_1,\dots,\hat{v}_n)\, \mathcal{V}_i[u]\, f_i + f_u. \tag{S91}$$

If the control is successful, the controlled wave equals approximately the uncontrolled wave profile $\mathbf{U}_c$ shifted according to the protocol follows its shifted wave profile and $u = U_c(x-\phi(t)) + \mathcal{O}(\epsilon)$, $v_i = V_c^i(x-\phi(t)) + \mathcal{O}(\epsilon)$ to leading order in $\epsilon$. With $U_c = U_c(x-\phi(t))$, $V_c^i = V_c^i(x-\phi(t))$ it follows

$$\begin{aligned}& \partial_{V_c^1} R\left(U_c, V_c^1,\dots,V_c^n\right) \mathcal{V}_1[U_c]\, \tilde{f}_1 \\ & = \sum_{i=1}^n \partial_{V_c^i} R\left(U_c, V_c^1,\dots,V_c^n\right) \mathcal{V}_i[U_c]\, f_i + f_u.\end{aligned} \tag{S92}$$

Solving for $\tilde{f}_1$ with the help of the inverse operator $\mathcal{V}_1^{-1}[U_c]$ of the Green's operator $\mathcal{V}_1[U_c]$,

$$\mathcal{V}_1^{-1}[U_c] = \partial_t - D_i \partial_x^2 - h_i(U_c), \tag{S93}$$

gives the final result

$$\begin{aligned}\tilde{f}_1 = {} & \mathcal{V}_1^{-1}[U_c]\left(\frac{\sum_{i=1}^n \partial_{V_c^i} R\left(U_c, V_c^1,\dots,V_c^n\right) \mathcal{V}_i[u]\, f_i}{\partial_{V_c^1} R\left(U_c, V_c^1,\dots,V_c^n\right)}\right) \\ & + \mathcal{V}_1^{-1}[U_c]\left(\frac{f_u}{\partial_{V_c^1} R\left(U_c, V_c^1,\dots,V_c^n\right)}\right).\end{aligned} \tag{S94}$$

## VI. POSITION CONTROL OF TW SOLUTIONS TO THE OREGONATOR MODEL FOR THE PHOTOSENSITIVE BZ REACTION

The model equations for the three component Oregonator model are

$$\partial_t u = D_u \partial_x^2 u + \frac{1}{\tilde{\epsilon}}\left(u - u^2 + w\left(q-u\right)\right) + \epsilon f_u, \quad \text{(S95)}$$

$$\partial_t v = u - v + \epsilon f_v, \quad \text{(S96)}$$

$$\partial_t w = D_w \partial_x^2 w + \frac{1}{\hat{\epsilon}}\left(\Phi_0 + f_0 v - w\left(q+u\right)\right) + \epsilon f_w. \quad \text{(S97)}$$

Here, $u$, $v$, $w$, denote the dimensionless concentrations of malonic acid, the oxydized form of the Ruthenium catalytic complex, and the inhibitor, respectively. The characteristic time scales$\hat{\epsilon}$, $\tilde{\epsilon}$ and the kinetic parameters $f_0$ and $q$ are assumed to be constant. The photochemically produced bromide flow $\Phi_0$ is proportional to the applied light sensitivity and can be controlled spatio-temporally in experiments. We show that our control method can be used to control the position of BZ waves.
First, we consider a constant $\Phi_0$ and non-zero control functions $f_u$, $f_v$, $f_w$. Then the solution for the control function is given as

$$\mathbf{f}\left(x,t\right) = \begin{pmatrix} f_u\left(x,t\right) \\ f_v\left(x,t\right) \\ f_w\left(x,t\right) \end{pmatrix} = \left(c - \dot{\phi}\left(t\right)\right)\mathbf{U}_c'\left(x-\phi\left(t\right)\right). \quad \text{(S98)}$$

The equations for $v$ and $w$ are linear in $v$ and $w$, respectively, i.e. their solutions can be written in terms of Green's functions. Both equations are linear inhomogeneous PDEs with initial conditions $v_0$, $w_0$,

$$\partial_t v + v = u + \epsilon f_v, \quad \text{(S99)}$$

$$v\left(x,t_0\right) = v_0\left(x\right), \quad \text{(S100)}$$

$$\partial_t w - D_w \partial_x^2 w + w\left(q+u\right)/\hat{\epsilon} = \frac{1}{\hat{\epsilon}}\left(\Phi_0 + f_0 v\right) + \epsilon f_w, \quad \text{(S101)}$$

$$w\left(x,t_0\right) = w_0\left(x\right). \quad \text{(S102)}$$

Their solutions can be written as

$$v\left(x,t\right) = \mathcal{K}\left(u + \epsilon f_v\right) + \mathcal{K}_0 v_0, \quad \text{(S103)}$$

$$w\left(x,t\right) = \mathcal{F}\left(\left(\Phi_0 + f_0 v\right)/\hat{\epsilon} + \epsilon f_w\right) + \mathcal{F}_0 w_0, \quad \text{(S104)}$$

with $\mathcal{K}$, $\mathcal{K}_0$, $\mathcal{F}$, $\mathcal{F}_0$ being Green's operators for the initial conditions ($\mathcal{K}_0$, $\mathcal{F}_0$) and for the inhomogeneity ($\mathcal{K}$, $\mathcal{F}$). The operators $\mathcal{F}$ and $\mathcal{F}_0$ depend on $u$ because of the term $\left(q+u\right)/\hat{\epsilon}$, so we should write

$$\mathcal{F} = \mathcal{F}\left[u\left(x,t\right)\right], \qquad \mathcal{F}_0 = \mathcal{F}_0\left[u\left(x,t\right)\right]. \quad \text{(S105)}$$

Additionally, operators depend on $\epsilon$ through $u$. The solution for $w$ can be written in terms of the solution for $v$ as

$$w\left(x,t\right) = \frac{\Phi_0}{\hat{\epsilon}}\mathcal{F} + \frac{f_0}{\hat{\epsilon}}\mathcal{F}\mathcal{K}u + \frac{f_0}{\hat{\epsilon}}\mathcal{F}\mathcal{K}_0 v_0 + \mathcal{F}_0 w_0 + \epsilon\mathcal{F}f_w + \epsilon\frac{f_0}{\hat{\epsilon}}\mathcal{F}\mathcal{K}f_v. \quad \text{(S106)}$$

The full Oregonator model can be written as a single nonlinear IDE for $u$,

$$\begin{aligned}\partial_t u = {} & D_u \partial_x^2 u + \frac{1}{\tilde{\epsilon}}\left(u - u^2\right) \\ & + \frac{1}{\tilde{\epsilon}}\left(q-u\right)\left(\frac{\Phi_0}{\hat{\epsilon}}\mathcal{F} + \frac{f_0}{\hat{\epsilon}}\mathcal{F}\mathcal{K}u + \frac{f_0}{\hat{\epsilon}}\mathcal{F}\mathcal{K}_0 v_0 + \mathcal{F}_0 w_0\right) \\ & + \frac{\epsilon}{\tilde{\epsilon}}\left(q-u\right)\left(\mathcal{F}f_w + \frac{f_0}{\hat{\epsilon}}\mathcal{F}\mathcal{K}f_v\right) + \epsilon f_u. \end{aligned} \quad \text{(S107)}$$

We compare Eq. (S107) with the experimentally realistic case of BZ waves controlled by a spatio-temporal light intensity acting on parameter $\Phi_0$ according to $\Phi_0 \to \Phi_0 + \epsilon\Phi\left(x,t\right)$. All other control terms are set to zero, $f_u \equiv f_v \equiv f_w \equiv 0$. The controlled Oregonator model is

$$\partial_t u = D_u \partial_x^2 u + \frac{1}{\tilde{\epsilon}}\left(u - u^2 + w\left(q-u\right)\right), \quad \text{(S108)}$$

$$\partial_t v = u - v, \quad \text{(S109)}$$

$$\partial_t w = D_w \partial_x^2 w + \frac{1}{\hat{\epsilon}}\left(\Phi_0 + f_0 v - w\left(q+u\right)\right) + \frac{\epsilon}{\hat{\epsilon}}\Phi. \quad \text{(S110)}$$

Similar as above, this can be written as a single IDE for the activator $u$

$$\begin{aligned}\partial_t u = {} & D_u \partial_x^2 u + \frac{1}{\tilde{\epsilon}}\left(u - u^2\right) \\ & + \frac{1}{\tilde{\epsilon}}\left(q-u\right)\left(\frac{\Phi_0}{\hat{\epsilon}}\mathcal{F} + \frac{f_0}{\hat{\epsilon}}\mathcal{F}\mathcal{K}u + \frac{f_0}{\hat{\epsilon}}\mathcal{F}\mathcal{K}_0 v_0 + \mathcal{F}_0 w_0\right) \\ & + \frac{\epsilon}{\hat{\epsilon}\tilde{\epsilon}}\left(q-u\right)\mathcal{F}\Phi. \end{aligned} \quad \text{(S111)}$$

Comparing the control terms to order $\mathcal{O}\left(\epsilon\right)$ in Eq. (S107) and Eq. (S111), we get

$$\frac{1}{\tilde{\epsilon}}\left(q - U_c\left(x-\phi\left(t\right)\right)\right)\left(\mathcal{F}^0 f_w + \frac{f_0}{\hat{\epsilon}}\mathcal{F}^0\mathcal{K}f_v\right) + f_u = \frac{1}{\hat{\epsilon}\tilde{\epsilon}}\left(q - U_c\left(x-\phi\left(t\right)\right)\right)\mathcal{F}^0\Phi. \quad \text{(S112)}$$

Here we introduced the operator $\mathcal{F}^0 = \mathcal{F}^0\left[U_c\left(x-\phi\left(t\right)\right)\right]$ which arises by expanding $\mathcal{F}\left[u\left(x,t\right)\right]$ up to $\mathcal{O}\left(\epsilon\right)$. The final solution for $\Phi\left(x,t\right)$ reads

$$\Phi\left(x,t\right) = \hat{\epsilon}f_w\left(x,t\right) + f_0 h\left(x,t\right) \quad \text{(S113)}$$

$$+ \mathcal{F}^{-0}\left(\frac{\hat{\epsilon}\tilde{\epsilon}}{\left(q - U_c\left(x-\phi\left(t\right)\right)\right)}f_u\left(x,t\right)\right). \quad \text{(S114)}$$

The operator $\mathcal{F}^{-0}$ is the inverse operator to $\mathcal{F}^0$ and given as

$$\mathcal{F}^{-0} = \partial_t - D_w\partial_x^2 + \left(q + U_c\left(x-\phi\left(t\right)\right)\right)/\hat{\epsilon}, \quad \text{(S115)}$$

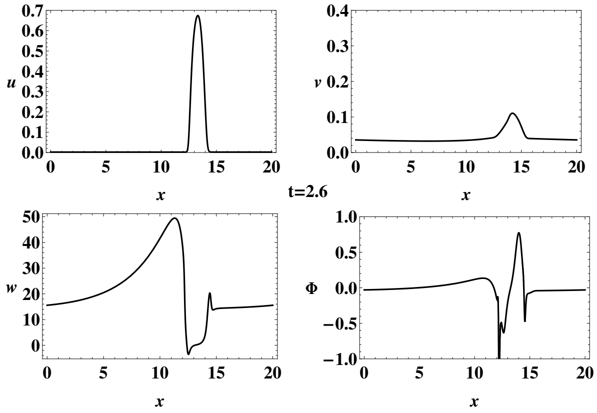


Figure S6. **S6.avi:** Position control via parameter $\Phi$ in the Oregonator model. Clockwise from top left: Activator $u$, catalyst $v$, inhibitor $w$ and control function $\Phi\left(x,t\right)$ proportional to applied light intensity. The control reverses the propagation direction. The profile of the catalyst $v$ is deformed while the activator $u$ and inhibitor $w$ are largely unaffected by the control.

while the term $h\left(x,t\right)=\mathcal{K}f_{v}\left(x,t\right)$ is the solution to the inhomogeneous PDE

$$\partial_{t}h+h=f_{v}, \tag{S116}$$
$$h\left(x,t_{0}\right)=0. \tag{S117}$$

The term $\frac{\hat{\epsilon}\tilde{\epsilon}}{\left(q-U_{c}\left(x-\phi\left(t\right)\right)\right)}$ does not diverge because $U_{c}\left(x\right)>q$ for all $x$.
With the values of the system parameters

$$\tilde{\epsilon}=1/35.5, \qquad \hat{\epsilon}=0.011\tilde{\epsilon}, \tag{S118}$$
$$f_{0}=1.16, \qquad \Phi_{0}=0.056, \tag{S119}$$
$$q=0.002, \qquad D_{u}=1, \tag{S120}$$
$$D_{w}=1.12. \tag{S121}$$

we obtain a velocity $c=3.384$ of the uncontrolled TW. The protocol

$$\phi\left(t\right)=ct\left(1-4t/3\right) \tag{S122}$$

reverses the propagation direction and eventually moves the pulse backward. Fig. S6 and the corresponding movie shows position control of the Oregonator model via parameter $\Phi$.

## VII. FAILURE OF POSITION CONTROL

We show an example for the failure of position control for the case of the controlled Oregonator model

$$\partial_{t}u=D_{u}\partial_{x}^{2}u+\frac{1}{\tilde{\epsilon}}\left(u-u^{2}+w\left(q-u\right)\right)+\epsilon f_{u}, \tag{S123}$$
$$\partial_{t}v=u-v+\epsilon f_{v}, \tag{S124}$$
$$\partial_{t}w=D_{w}\partial_{x}^{2}w+\frac{1}{\hat{\epsilon}}\left(\Phi_{0}+f_{0}v-w\left(q-u\right)\right)+\epsilon f_{w}. \tag{S125}$$

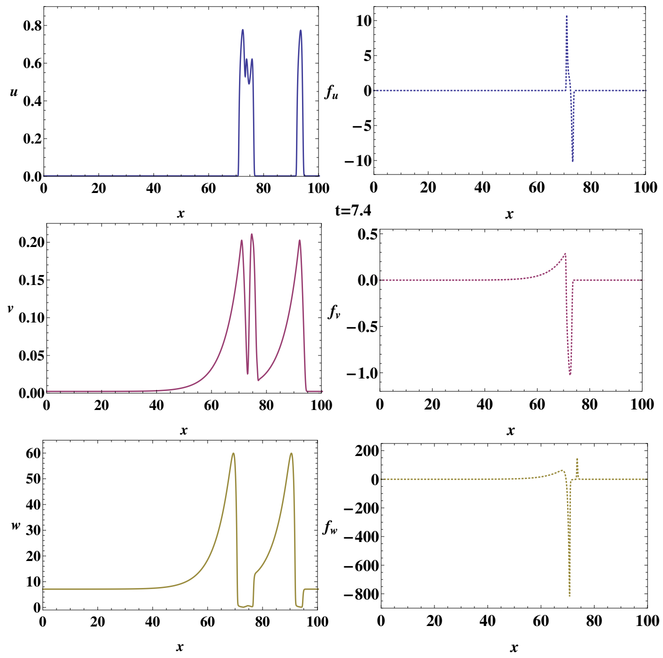


Figure S7. **S7.avi:** Position control of a traveling pulse solution of the Oregonator model. Left windows show the pulse profiles of $u$, $v$, $w$ (from top to bottom). The corresponding control functions are shown in the right windows. The pulse follows the decelerating protocol until the control functions become too large and pulses are emitted to the right in an irregular fashion.

The control functions are given as

$$\mathbf{f}\left(x,t\right)=\begin{pmatrix}f_{u}\left(x,t\right)\\ f_{v}\left(x,t\right)\\ f_{w}\left(x,t\right)\end{pmatrix}=\left(c-\dot{\phi}\left(t\right)\right)\mathbf{U}_{c}'\left(x-\phi\left(t\right)\right). \tag{S126}$$

We choose a protocol which decreases the velocity

$$\phi\left(t\right)=ct\left(1-\alpha t\right), \qquad \alpha=\frac{1}{10}. \tag{S127}$$

The model parameter values are

$$q=0.002, \qquad f_{0}=1.4, \qquad \tilde{\epsilon}=1/40, \tag{S128}$$
$$\hat{\epsilon}=1/3600, \qquad \Phi_{0}=0.0275, \qquad D_{u}=1.0, \tag{S129}$$
$$D_{w}=1.12. \tag{S130}$$

The velocity $c$ of the uncontrolled stable pulse solution is

$$c=5.765. \tag{S131}$$

Shortly before the velocity of the protocol changes sign, the TW is destroyed and pulses are emitted to the right, see Fig. S7. Compare this result with the case of position control via the parameter $\Phi_{0}$ proportional to the light intensity, Fig. S6, where a traveling pulse is successfully moved backward and no pulses are emitted to the right.

## VIII. STATIONARY CONTROL

### A. Solution to the Fredholm integral equation of the first kind

For stationary control of TW solutions to a single component RDS we formulated a Fredholm integral equation of the first kind for the unknown control $f(x)$ in the form

$$g(\phi) = \int_{-\infty}^{\infty} K(\phi - x) f(x) dx. \tag{S132}$$

$g(\phi)$ and $K(\phi - x)$ are known as inhomogeneity and kernel, respectively. In the following we give some details of the calculations leading to a solution $f(x)$ to Eq. (S132). The idea is to apply the convolution theorem for integral transforms to convert the convolution Eq. (S132) to an algebraic equation. We will apply the bilateral Laplace transform, also called two-sided Laplace transform, of a function $f$, which is defined as (see e.g. [10])

$$F(s) = \mathcal{L}\{f(t)\} = \int_{-\infty}^{\infty} dt e^{-st} f(t). \tag{S133}$$

Here $s \in \mathbb{C}$ and therefore Eq. (S133) can also be seen as a generalized Fourier transform for complex (instead of purely imaginary) frequency $s$. The Laplace transform is defined by two entities: the algebraic expression for $F(s)$ and the region of convergence (ROC), e.g. the range of complex $s$ values where $F(s)$ exists. The ROC is defined as

$$\text{ROC} = \left\{ s = \sigma + i\omega \,\text{so that} \int_{-\infty}^{\infty} dt \left| e^{-\sigma t} f(t) \right| < \infty \right\}. \tag{S134}$$

The ROC is a strip parallel to the imaginary axis of finite width. The inverse bilateral Laplace transform is given by the Bromwich integral

$$f(t) = \frac{1}{2\pi i} \int_{\sigma - i\infty}^{\sigma + i\infty} ds F(s) e^{st}, \tag{S135}$$

where the value of ($\Re(z)$ denotes the real part of $z$) $\sigma = \Re(s)$ for the contour integral must be in the region of convergence.
The convolution theorem for the bilateral Laplace transform can be proven with the help of the change of variables $\phi = u + v$, $x = v$,

$$\begin{aligned}
\mathcal{L}\{g(\phi)\} &= \int_{-\infty}^{\infty} d\phi e^{-s\phi} \int_{-\infty}^{\infty} dx K(\phi - x) f(x) \\
&= \int_{-\infty}^{\infty} du \int_{-\infty}^{\infty} dv e^{-s(u+v)} K(u) f(v) \\
&= \int_{-\infty}^{\infty} du e^{-su} K(u) \int_{-\infty}^{\infty} dv e^{-sv} f(v) \\
&= \mathcal{L}\{K(u)\} \cdot \mathcal{L}\{f(u)\}.
\end{aligned} \tag{S136}$$

This allows us to write

$$\mathcal{L}\{f(x)\} = \frac{\mathcal{L}\{g(\phi)\}}{\mathcal{L}\{K(u)\}} \tag{S137}$$

and applying the inverse Laplace transform yields a general result for the control function $f$

$$f(x) = \frac{1}{2\pi i} \int_{\sigma - i\infty}^{\sigma + i\infty} ds \frac{\mathcal{L}\{g(\phi)\}}{\mathcal{L}\{K(u)\}} e^{sx} \tag{S138}$$

where the value of $\sigma$ must be in the region of convergence of both $\mathcal{L}\{g(\phi)\}$ and $\mathcal{L}\{K(u)\}$.
To evaluate the integral in Eq. (S138) we need to be more specific and choose a certain model and protocol. The Schlögl model

$$\partial_t u = \partial_x^2 u + R(u) \tag{S139}$$

has a cubic reaction function

$$R(u) = -u(u - a)(u - 1), \; -\frac{1}{2} < a < \frac{1}{2} \tag{S140}$$

with TW solution

$$U_c(\xi) = \frac{1}{1 + \exp\left(\xi/\sqrt{2}\right)} \tag{S141}$$

and velocity

$$c = \frac{1}{\sqrt{2}}(1 - 2a). \tag{S142}$$

The kernel $K(x)$ is given as

$$K(x) = e^{-cx} U_c(-x), \tag{S143}$$

and the constant $K_c$ can be determined as

$$\begin{aligned}
K_c &= \int_{-\infty}^{\infty} dx e^{cx} \left(U_c'(x)\right)^2 \\
&= \frac{1}{6}\pi c\left(1 - 2c^2\right) \csc\left(\sqrt{2}\pi c\right).
\end{aligned} \tag{S144}$$

Note that the velocity is restricted to

$$-\frac{1}{\sqrt{2}} < c < \frac{1}{\sqrt{2}} \tag{S145}$$

because $a$ is restricted to $-1/2 < a < 1/2$. The bilateral Laplace transform of the kernel $K$ is

$$\mathcal{L}\left\{K\left(u\right)\right\} = -\sqrt{2}\pi\left(c+s\right)\csc\left(\sqrt{2}\pi\left(c+s\right)\right), \tag{S146}$$

with a ROC given by

$$-\frac{1}{\sqrt{2}} < c + \Re\left(s\right) < \frac{1}{\sqrt{2}}. \tag{S147}$$

We choose $\phi\left(t\right)$ so that

$$\phi'\left(t\right) = \frac{c}{2}\left(1+\tanh\left(k\left(t_1-t\right)\right)\right),\ t_1 > t_0,\ k>0 \tag{S148}$$

which is a smooth representation of the Heaviside Theta function $c\Theta\left(t\right)$,

$$\Theta\left(t\right) = \lim_{k\to\infty}\frac{1}{2}\left(1+\tanh\left(kt\right)\right) = \lim_{k\to\infty}\frac{1}{1-e^{-2kt}}. \tag{S149}$$

So for $t\to-\infty$, the velocity $\phi'\left(t\right)$ equals the velocity $c$ of the unperturbed case, for $t\to\infty$, the velocity is zero. At time $t_1$, the acceleration is maximal, and in the limit $k\to\infty$, the front is stopped at time $t_1$. For $\phi\left(t\right)$ together with the initial condition Eq. $\phi\left(t_0\right) = \phi_0$ we find

$$\phi\left(t\right) = \phi_0 + \frac{c}{2}\left(t-t_0\right) + \frac{c}{2k}\log\left(\frac{\cosh\left(k\left(t_0-t_1\right)\right)}{\cosh\left(k\left(t-t_1\right)\right)}\right). \tag{S150}$$

We can invert $\phi\left(t\right)$ to obtain $T\left(\phi\right)$ and find for the inhomogeneity $g$

$$\begin{aligned} g\left(\phi\right) &= K_c\left(c - \frac{1}{T'\left(\phi\right)}\right) \\ &= K_c\frac{c\exp\left(\frac{2k}{c}\left(ct_0+\phi-\phi_0\right)\right)}{e^{2kt_0}+e^{2kt_1}}\Theta\left(\phi-\phi_0\right). \end{aligned} \tag{S151}$$

We include the Heaviside Theta function $\Theta\left(\phi-\phi_0\right)$ in the definition of $g$ to remind us that the perturbation $f\left(x\right)$ is switched on at time $t_0$, and so the protocol $\phi\left(t\right)$ is not defined at earlier times. For all times $t \leq t_0$, the front moves with the velocity $c$ of the unperturbed case. If $\Theta\left(\phi-\phi_0\right)$ is neglected in the definition of $g\left(\phi\right)$, its Laplace transform does not exist. For the bilateral Laplace transform of $g\left(\phi\right)$ we find

$$\mathcal{L}\left\{g\left(\phi\right)\right\} = K_c\frac{c^2e^{2kt_0-s\phi_0}}{\left(e^{2kt_0}+e^{2kt_1}\right)\left(cs-2k\right)}, \tag{S152}$$

with a ROC given by

$$2k < c\Re\left(s\right). \tag{S153}$$

The ROC is the right half complex plane with the real part of $s$ larger than $2k/c$. Combining the two conditions for the existence of the Laplace transforms, Eqs. (S147) and (S153), we find a condition for $k$ (we assume a front traveling to the right so that $c>0$)

$$0 < k < \frac{c\Re\left(s\right)}{2} < \frac{c}{2}\left(\frac{1}{\sqrt{2}}-c\right). \tag{S154}$$

The next step is to compute the integral arising in the general solution Eq. (S138)

$$\begin{aligned} f\left(x\right) &= \frac{1}{2\pi i}\int_{\sigma-i\infty}^{\sigma+i\infty} ds\frac{\mathcal{L}\left\{g\left(\phi\right)\right\}}{\mathcal{L}\left\{K\left(u\right)\right\}}e^{sx} \\ &= -\frac{K_c}{2\pi i}\frac{c^2e^{2kt_0}}{\sqrt{2}\pi\left(e^{2kt_0}+e^{2kt_1}\right)}\times \\ &\int_{\sigma-i\infty}^{\sigma+i\infty} ds\frac{\sin\left(\sqrt{2}\pi\left(c+s\right)\right)}{\left(cs-2k\right)\left(c+s\right)}e^{s\left(x-\phi_0\right)}, \end{aligned} \tag{S155}$$

$$\frac{2k}{c} < \sigma = \Re\left(s\right) < \frac{1}{\sqrt{2}} - c. \tag{S156}$$

In principle this integral can be solved with the help of the Residue theorem, which involves the determination of the poles of the integrand. The pole at $s = -c$ is not a real pole, since the integrand behaves as $\lim_{x\to0}\sin\left(x\right)/x$, and the residue at this point is 0. The residue at $s = \frac{2k}{c}$ is

$$\begin{aligned} &\mathrm{Res}\left(\frac{\sin\left(\sqrt{2}\pi\left(c+s\right)\right)}{\left(cs-2k\right)\left(c+s\right)}e^{s\left(x-\phi_0\right)}, s=\frac{2k}{c}\right) \\ &= \frac{\sin\left(\frac{\sqrt{2}\pi}{c}\left(c^2+2k\right)\right)\exp\left(\frac{2k}{c}\left(x-\phi_0\right)\right)}{c^2+2k}. \end{aligned} \tag{S157}$$

As a first guess, we suspect that the value of the integral Eq. (S155) is solely given by $2\pi i$ times the residue at $s = 2k/c$. This yields a solution for the control function

$$f\left(x\right) = -\frac{K_cc^2\sin\left(\frac{\sqrt{2}\pi}{c}\left(c^2+2k\right)\right)\exp\left(\frac{2k}{c}\left(x-\phi_0\right)\right)}{\sqrt{2}\pi\left(1+e^{2k\left(t_1-t_0\right)}\right)\left(c^2+2k\right)}. \tag{S158}$$

To confirm our first guess, we prove that this is a valid solution of the inverse problem by solving the regular problem, i.e. we solve the equation of motion, Eq. (4) of the main text, for $\phi\left(t\right)$ with the control function given by Eq. (S158).

### B. Regularization of the control solution

The solution for the control $f\left(x\right)$, Eq. (S158), diverges for large $x$,

$$\lim_{x\to\infty} f\left(x\right) = -\infty. \tag{S159}$$

A diverging control destroys the TW and therefore the solution must be regularized. One possibility is to simply cut off the control at specified values $f_{\min}$, $f_{\max}$ such that

$$f_{\min} \le f(x) \le f_{\max}. \tag{S160}$$

In the main text, we applied the simple criterion of local bistability to determine $f_{\min}$ and $f_{\max}$. We consider a rescaled Schlögl model with a constant $f_{\text{const}}$

$$\partial_t u = \partial_x^2 u + R(u) + f_{\text{const}}, \tag{S161}$$

with $R(u)$ given by Eq. (S140). Front solutions to this model do only exist as long Eq. (S161) does possess three different homogeneous steady states. Therefore the cubic polynomial for $u$,

$$-u(u-a)(u-1) + f_{\text{const}} = 0 \tag{S162}$$

must have have three different real roots. This condition can only be fulfilled for a certain range of possible values for $f_{\text{const}}$,

$$f_{\min} \le f_{\text{const}} \le f_{\max}. \tag{S163}$$

The parameter $f_{\min}$ ($f_{\max}$) can be determined as the local minimum (maximum) of $R(u)$ given by $R(u_{\min})$ ($R(u_{\max})$), where $u_{\min}$ ($u_{\max}$) are the roots of the quadratic polynomial $R'(u) = 0$. We find

$$\begin{aligned} f_{\min} &= R(u_{\min}) \\ &= \frac{1}{27}\left(-2 + 3a + 3a^2 - 2a^3 - 2\left(a^2 - a + 1\right)^{3/2}\right), \end{aligned} \tag{S164}$$

$$\begin{aligned} f_{\max} &= R(u_{\max}) \\ &= \frac{1}{27}\left(-2 + 3a + 3a^2 - 2a^3 + 2\left(a^2 - a + 1\right)^{3/2}\right). \end{aligned} \tag{S165}$$

For the Schlögl model with a spatially varying perturbation $f(x)$,

$$\partial_t u = \partial_x^2 u - u(u-a)(u-1) + f(x), \tag{S166}$$

we can apply the same condition: the existence of (slightly deformed) front solutions to Eq. (S166) is guaranteed as long as bistability is preserved at every point $x$ in space,

$$f_{\min} \le f(x) \le f_{\max}. \tag{S167}$$

This gives a very conservative estimate, and usually the front profile is not deformed very much if this condition is violated within a small spatial interval.

A different possibility to regularize the control function $f(x)$ would be to consider the constraint Eq. (S167) from the very beginning. One could try to find a solution to the constrained integral equation

$$g(\phi) = \int_{-\infty}^{\infty} K(\phi - x) f(x)\, dx, \tag{S168}$$

$$f_{\min} \le f(x) \le f_{\max}. \tag{S169}$$

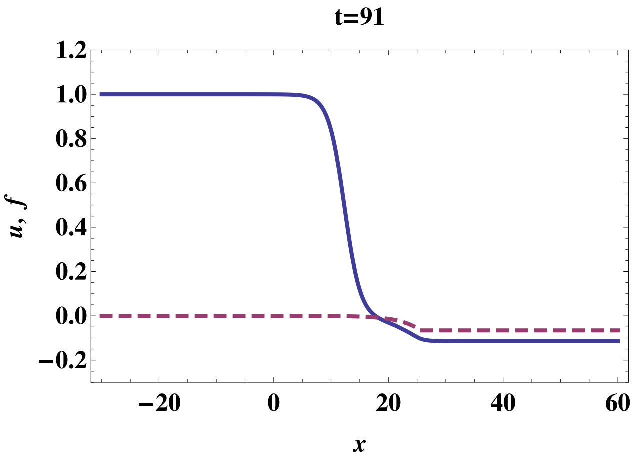


Figure S8. **S8.avi:** Stationary control of a Schlögl front solution (blue solid line). The front is stopped and the front profile becomes slightly deformed when it enters the region where the absolute value of the control (purple dashed line) is large.

It is possible to transform a Fredholm integral equation to the problem of minimizing a squared difference. Furnished with the constraint Eq. (S169), we obtain a constrained minimization problem. Note that the problem of finding an optimal control is also constrained minimization problem, and so similar numerical algorithms can be applied. There are a couple of numerical methods to solve constrained minimization problems, see e.g. [11, 12].

### C. Comparison with numerical simulations

For numerical simulations of the controlled Schlögl, we choose

$$a = 0.4 \tag{S170}$$

for the value of the system parameter $a$. The velocity $c$ of the uncontrolled front solution is

$$c = \frac{1}{\sqrt{2}}(1 - 2a) = 0.141. \tag{S171}$$

For the velocity protocol decelerating the front solution we choose

$$\dot{\phi}(t) = \frac{c}{2}\left(1 + \tanh\left(k\left(t_1 - t\right)\right)\right), \; t_1 > t_0, \; k > 0, \tag{S172}$$

with protocol parameters

$$t_0 = 0, \qquad \phi_0 = 0, \tag{S173}$$

$$t_1 = 130, \qquad k = \frac{1}{2}k_{\max} = 0.02. \tag{S174}$$

See a snapshot of the front evolution under stationary control in Fig. S8 and corresponding movie. Because

the control function is not proportional to the Goldstone mode $U_c'(x)$, the front profile becomes slightly deformed when it enters the region where the absolute value of the control is large.

---

[1] J. Löber, M. Bär, and H. Engel, Phys. Rev. E **86**, 066210 (2012).
[2] F. Schlögl, Z. Phys. A **253**, 147 (1972).
[3] R. FitzHugh, Biophysical J. **1**, 445 (1961); J. Nagumo, S. Arimoto, and S. Yoshizawa, Proc. IRE **50**, 2061 (1962).
[4] J. D. Murray, *Mathematical biology*, Vol. 3 (Springer-Verlag, Berlin, 1993).
[5] R. Fisher, Ann. Eugenics **7**, 355 (1937).
[6] A. Kolmogorov, I. Petrovsky, and N. Piskunov, Bull. Univ. Moscow, Ser. Int. A **1**, 1 (1937).
[7] U. Ebert and W. van Saarloos, Phys. Rev. Lett. **80**, 1650 (1998).
[8] W. van Saarloos, Phys. Rep. **301**, 9 (1998).
[9] A. L. Hodgkin and A. F. Huxley, J. Physiol. **117**, 500 (1952).
[10] J. L. Schiff, *The Laplace transform: theory and applications* (Springer-Verlag, Berlin, 1999).
[11] E. Babolian and L. Delves, IMA Journal of Applied Mathematics **24**, 157 (1979).
[12] J. Nocedal and S. J. Wright, *Numerical optimization* (Springer New York, 1999).
